# Supplementary material for: Verification of a real-time ensemble-based method for updating earth model based on GAN
Source: arXiv:2207.03596 source file (2022-07-07)
Supplement: Supplementary file 1 [file appendix.tex]

\section{Appendix: geological setting and training data for the GAN}
\label{sec:geosetting}
\label{sec:appendix}

For training of GAN we use a large (compare to the area of prediction) reference geo-model,
which should provide a realistic test case for the present study in terms of scale and actual geological features and properties.
% as rendered in standard reservoir models.  
Key requirements included: (1) the model should be built using an industry-standard reservoir modeling software; (2) it should cover several square kilometers and have  vertical extent of a few hundred meters; (3) high grid resolution; (4) moderate to high geologic complexity; (5) depositional architectures consisting of lithologies with contrasting resistivity; 
%was porosity
(6) for ease of handling and analysis of test results, structural elements such as faults and fractures should not be included.

In order to fulfill these requirements, the we use a commercial software to construct a base geo-model that comprises a synthetic structural framework, a facies model set-up derived from outcrop analogue data, and synthetic petrophysical properties of individual facies derived from published literature. 
% The model was constructed using RMS\textsuperscript{TM} 11.0.1 supplied by Emerson/Roxar~\cite{Emers}. 
The resulting base model employs a local coordinate system and measures 4000m x 1000m x 200m (xyz).
Cell dimensions were set to 10x10x0.5 m yielding a regularized corner-point grid measuring 400 x 100 x 400 cells (xyz).

\subsection{Facies model}
%Model requirements regarding moderate- to high-complexity and lithology architectures with contrasting porosity/resistivity can be fulfilled by several different depositional architectures exhibiting layered stratigraphy with contrasting properties. For the present study
A low net/gross fluvial system was chosen as the depositional architecture since it provides complex 3D architectures comprising a limited number of facies exhibiting contrasting 
% porosity and 
geometries.  

Input numbers for facies dimensions and geometry are derived from a well-documented outcrop of the Cretaceous lower Williams Fork Formation (Mesa Verde Group) at Coal Canyon, Colorado, USA.~\cite{Pranter2014,Pranter2011,Trampush2017}.
%The outcrop consists of a 1500 m wide and 200 m thick succession of fluvial and overbank sediments deposited in a coastal plain setting of foreland basin under warm temperate climate conditions. 
%
Key parameters of the facies model set-up are listed in Table~\ref{tab:tab1}. The model is not intended as a rendering of the outcrop itself and is consequently somewhat simplified compared to descriptions of the outcrop provided by~\cite{Cole2005,Panjaitan2006,Pranter2009,Pranter2011}.
%and the requirements listed above.  

The model contains three facies: Background/shale, Channels and Crevasse splays. 
% Although three different channel types (Single story channel, narrow channel body and multi-story channel) are described from the outcrop,
% The model set-up is restricted to single story channels. 
The probability distribution of channel width in the model is adapted to include “narrow channel bodies”, and stacking of channels accounts for multi-story channels which comprise more than 80\% of the observed channel bodies. The flow direction of the channel system is set towards $45 \pm 10$ degrees. No trends were used to condition the spatial distribution of channels.  
% Defining the map-view geometry of crevasse splays from outcrop data is difficult. Using thickness and volumetric proportion of crevasse splays as a guideline, the remaining parameter settings where adjusted heuristically. 

\begin{table}
\caption{Parameter settings for facies models.}\label{tab:tab1}
\begin{tabular}{|l|l|l|l|}
\hline
\underline{Volumetric fraction} & Value & Tolerance & Comments\\
\hline
Channel system volume fraction &  0.3 & 0.05 & \\
Channel positioning &  1 & & No trends \\
  Crevasse volume fraction & 0.1 & 0.03 & Of channel system vol. frac. \\
  \hline
\end{tabular}
%\vspace{0.1cm}
\begin{tabular}{|l|l|l|l|l|}
\hline
\underline{Channel geometry} & Value & SD & Min. & Max.\\
\hline
  Thickness & 4.2 & 1.5 & & \\
  Width & 155 & 50 & 20 & 500 \\
  Correlation W/T & 36 & & & \\
  Amplitude & 400 & 50 & & \\
  Sinuosity & 1.3 & & & \\
  Azimuth & 45 & 10 & & \\
  \hline
\end{tabular}
%\vspace{0.1cm}
\begin{tabular}{|l|l|}
\hline
\underline{Form/repulsion} & Setting  \\
\hline
  Cross-section geometry & Parabolic, basic variability \\
  Channel form & Rigid \\
  Repulsion & None \\
  \hline
\end{tabular}
%\vspace{0.1cm}
% \begin{tabular}{|l|l|l|l|}
% \hline
% \underline{Crevasse} & Value & SD & Comment \\
% \hline
%   Crevasse geometry & Isolated & & No continuous belts \\
%   Relative thickness & 0.3 & 0.1 & Of channel  \\
%   Channel margin coverage & 0.5 & & \\
%   Relative lobe width normal to channel & 0.7 & & \\
%   Absolute lobe length parallel to channel & 200 & & \\
%   Min. \# of crev. belts per channel & 2 & & \\
%   Max. \# of crev. belts per channel & 6 & & \\
%   Vertical position & Towards top & & \\
%   \hline
% \end{tabular}
\end{table}

% Porosity and porosity contrasts of the Williams Fork Fm. are very low, e.g.,~\cite{Pranter2011}, and thus for our purpose. 

% \begin{table}[]
%     \centering
%     \begin{tabular}{|r|l|r|}
%     \hline
%         Index & Facies & $R$ \\
%     \hline
%          0 & Background & 220.0 \\
%          1 & Channel & 3.6 \\
%          2 & Crevasse & 4.1 \\
%     \hline
%     \end{tabular}
%     \caption{Resistivities of for different facies within the geomodel.}
%     \label{tab:resistivities}
% \end{table}

% \begin{table}
%   \caption{Facies model setup. *channel variograms follow body curvature. **crevasse variograms follow body direction. 
% %   Vertical trends are employed for Channel and Crevasse with porosity decreasing and increasing upward respectively.
%   }
%   \label{tab:tab2}
%   \begin{tabular}{|l|r|r|r|r|r|r|}
%     \hline
%     Facies 
%     & $R$ & Var.range parallel& Var. range normal & Var. range vertical & Direction & Dip\\
%     \hline
%     Background & 3.6 & 1000 & 500 & 10 & 45 & 0 \\
%     Channel & 220.0 & 400 & 200 & 1 & * & 0 \\
%     Crevasse & 4.0 & 60 & 30 & 1 & ** 90 & 0 \\
%     \hline 
%   \end{tabular}
% \end{table}
